# Supplementary material for: MaIL: A Unified Mask-Image-Language Trimodal Network for Referring Image Segmentation
Source: arXiv:2111.10747 source file (2021-11-25)
Supplement: Supplementary file 1 [file 8-appendix.tex]

\section{Appendix}
\subsection{Datasets and Evaluation Metrics}

We evaluate our proposed method on three commonly used benchmark datasets for referring image segmentation, including RefCOCO~\cite{yu2016modeling}, RefCOCO+~\cite{yu2016modeling} and G-Ref~\cite{mao2016generation, nagaraja2016modeling}.

\textbf{RefCOCO/RefCOCO+}~(UNC/UNC+) are two of the largest datasets for this task. Concretely, the RefCOCO dataset has 142,209 referring expressions for 50,000 objects in 19,994 images. And the RefCOCO+ dataset contains 19,992 images with 141,564 referring expressions for 49,856 objects in them. Another difference is that the absolute location descriptions are forbidden in RefCOCO+, which makes it more challenging compared to the RefCOCO dataset.

\textbf{G-Ref} dataset is collected from MSCOCO via the Amazon's Mechanical Turk. It contains 104,560 expressions referring to 54,822 objects in 26,711 images. It is notable that there exist two partitionings: the UMD partitioning~\cite{nagaraja2016modeling} which splits the dataset into train, validation and test set, and the Google partitioning~\cite{mao2016generation} which has only train and validation set publicly released. We evaluate our method on both partitionings.

\textbf{Evaluation Metrics.}
We use the mask intersection-over-union~(IoU) and Precision@$X$ as evaluation metrics. IoU is the intersection area divided by the union areas, which measures the overall performance of generated masks. The Precision@$X$ is the percentage of prediction masks whose IoU scores are higher than the given threshold X, where $X \in \left\{0.5, 0.6, 0.7, 0.8, 0.9\right\}$.

\subsection{Full Experiment Results}
We provide overall results of our \netname\ in two types of resolution configurations in Table~\ref{tab:supp_fullresults}, including all the aforementioned evaluation metrics, IoU and Prec@$X$.

\subsection{More Ablation study}

\begin{table}[h]
    \centering
    \small
    \setlength{\tabcolsep}{1.5mm}
    \begin{tabular}{@{}ccccccc@{}}
    \toprule
         Model
         & Pr@$0.5$ & Pr@$0.6$ & Pr@$0.7$ & Pr@$0.8$ & Pr@$0.9$ & IoU \\
    \midrule
       R-50 & \textbf{72.35} & \textbf{67.79} & \textbf{60.54} & \textbf{45.82} & \textbf{15.29} & \textbf{62.23} \\
       \midrule
       R-101 & 72.34 & 66.95 & 58.40 & 42.41 & 14.17 & 62.10 \\
    \bottomrule
    \end{tabular}
    \caption{Ablation study of off-the-shelf instance segmentation models.}
    \label{tab:supp_segmodel}
\end{table}

\textbf{Different off-the-shelf segmentation models} can affect experiment results. However, in our study we find the influence is incremental. We use two instance segmentation models: Mask R-CNN~\cite{he2017mask} with ResNet-50 and ResNet-101 backbone, all pre-trained on instances in train splits of RefCOCO/RefCOCO+/G-Ref, the model with ResNet-101 backbone is trained in a 3$\times$ schedule following the common setting.

The comparison results on the validation set of the RefCOCO+ dataset is shown in Tab.~\ref{tab:supp_segmodel}, results from two models only have a minor difference. We claim that is because we combine the features from mask and image modalities inside the network. And our segmentation head can play a role in refining the final segmentation result, thus utilizing different segmentation models only leads to little influence on final results. On the other hand, the mask modality can boost the performance as long as the segmentation model generates appropriate candidate masks. Here in our proposed \netname\ we simply want masks as an additional modality to provide focus on instance-level features, so we directly adapt Mask R-CNN with ResNet-50 backbone as our default segmentation model for mask generation, other different segmentation models may further promote the performance.

\begin{table}[h]
    \centering
    \small
    \setlength{\tabcolsep}{0.5mm}
    \begin{tabular}{@{}ccccccc@{}}
    \toprule
         $s_k$ origin
         & Pr@$0.5$ & Pr@$0.6$ & Pr@$0.7$ & Pr@$0.8$ & Pr@$0.9$ & IoU \\
    \midrule
       Mask features & 71.04 & 65.55 & 58.32 & 44.41 & 14.66 & 61.39 \\
       \midrule
       Image features & \textbf{72.35} & \textbf{67.79} & \textbf{60.54} & \textbf{45.82} & \textbf{15.29} & \textbf{62.23} \\
    \bottomrule
    \end{tabular}
    \caption{Ablation study of using different features to generate mask's score.}
    \label{tab:supp_maskscore}
\end{table}

\textbf{Mask score's generation} in our \netname\ is based on the image features from each mask's corresponding areas. We also test directly using masks' features from transformer encoder to generate corresponding scores. Given $\mathbf{F}_M=\left\{\mathbf{F}_M^K\right\}$, we directly conduct average pooling on features of each mask feature map and an MLP layer to generate score $s_k^{'}$ for each mask in this case:

\begin{equation}
    \mathbf{f}_k^{'} = \texttt{AVG}(\mathbf{F}_M^k),\quad s_k^{'} = \texttt{MLP}(\mathbf{f}_k^{'}).
\end{equation}

We compare the results of \netname\ and this variant in Tab.~\ref{tab:supp_maskscore}. By using mask's feature to generate scores, network's IoU performance will drop ~1\%, and 1\%-3\% on other metrics. We attribute this performance degradation to the fact that features from different masks are not in a common shared embedding space and thus can't guarantee a fair comparison as mentioned in decoder part. Our adaptive mask selection strategy selects proper mask features depending on scores from image features in each mask's corresponding area.

\begin{table*}[ht]
   \centering
   \small
   \setlength{\tabcolsep}{2.8mm}{\begin{tabular}{@{}clccccccc@{}}
      \toprule
      \multicolumn{3}{c}{} & \multicolumn{1}{c}{IoU} & \multicolumn{1}{c}{Pr@0.5} & \multicolumn{1}{c}{Pr@0.6} & \multicolumn{1}{c}{Pr@0.7} & \multicolumn{1}{c}{Pr@0.8} & \multicolumn{1}{c}{Pr@0.9} \\
      \midrule
      \multirow{9}{*}{\makecell[c]{MaIL\\(416$\times$416)}} 
      & \multirow{3}{*}{RefCOCO} 
      & val   & 69.38 & 81.61 & 76.31 & 68.82 & 50.76 & 16.67 \\
      & & testA & 71.31 & 84.35 & 79.81 & 71.86 & 54.22 & 14.92 \\
      & & testB & 66.76 & 76.64 & 70.71 & 61.76 & 48.33 & 19.42 \\
      \cmidrule{2-9}
      & \multirow{3}{*}{RefCOCO+}
      & val   & 61.02 & 70.82 & 65.76 & 58.40 & 42.72 & 13.02 \\
      & & testA & 64.68 & 75.92 & 71.00 & 63.15 & 47.22 & 12.86 \\
      & & testB & 54.86 & 61.84 & 56.48 & 49.34 & 37.26 & 14.22 \\
      \cmidrule{2-9}
      & \multirow{3}{*}{G-Ref} 
      & val~(U)  & 60.86 & 70.75 & 64.94 & 56.07 & 39.10 & 12.88 \\
      & & test~(U) & 61.39 & 71.14 & 65.46 & 56.28 & 39.71 & 12.63 \\
      & & val~(G)  & 60.26 & 69.82 & 65.26 & 57.66 & 42.15 & 14.27\\
      
      \midrule
      
      \multirow{9}{*}{MaIL} 
      & \multirow{3}{*}{RefCOCO} 
      & val   & 70.13 & 81.80 & 77.29 & 70.05 & 53.57 & 19.01 \\
      & & testA & 71.71 & 84.76 & 81.08 & 72.72 & 55.86 & 16.69 \\
      & & testB & 66.92 & 76.66 & 70.69 & 62.75 & 49.06 & 21.59 \\
      \cmidrule{2-9}
      & \multirow{3}{*}{RefCOCO+}
      & val   & 62.23 & 72.35 & 67.79 & 60.54 & 45.82 & 15.29 \\
      & & testA & 65.92 & 77.81 & 73.17 & 65.22 & 48.89 & 13.75 \\
      & & testB & 56.06 & 63.08 & 58.17 & 51.16 & 39.45 & 16.36 \\
      \cmidrule{2-9}
      & \multirow{3}{*}{G-Ref} 
      & val~(U)  & 62.45 & 72.24 & 67.33 & 58.83 & 42.58 & 14.15 \\
      & & test~(U) & 62.87 & 72.80 & 67.50 & 58.72 & 42.80 & 14.33 \\
      & & val~(G)  & 61.81 & 71.79 & 67.47 & 59.85 & 44.53 & 15.15 \\
      
      \bottomrule
   \end{tabular}}%
   \caption{Full results of our proposed \netname\ on all datasets with two resolution configurations.}
  %\vspace{-0.1in}
   \label{tab:supp_fullresults}%
\end{table*}%

\subsection{Visualization}

In this section, we show the visualization of the attention maps from our transformer encoder. As shown in Fig.~\ref{fig:vis_attn}, given query as the ground truth location in image, together with the increasing of encoder's layer depth, the attention map of the whole image gradually focuses on the desired area, meanwhile the attention for other disruptive regions decreases.

\begin{figure*}[h]
  \centering
  \includegraphics[width=0.95\linewidth]{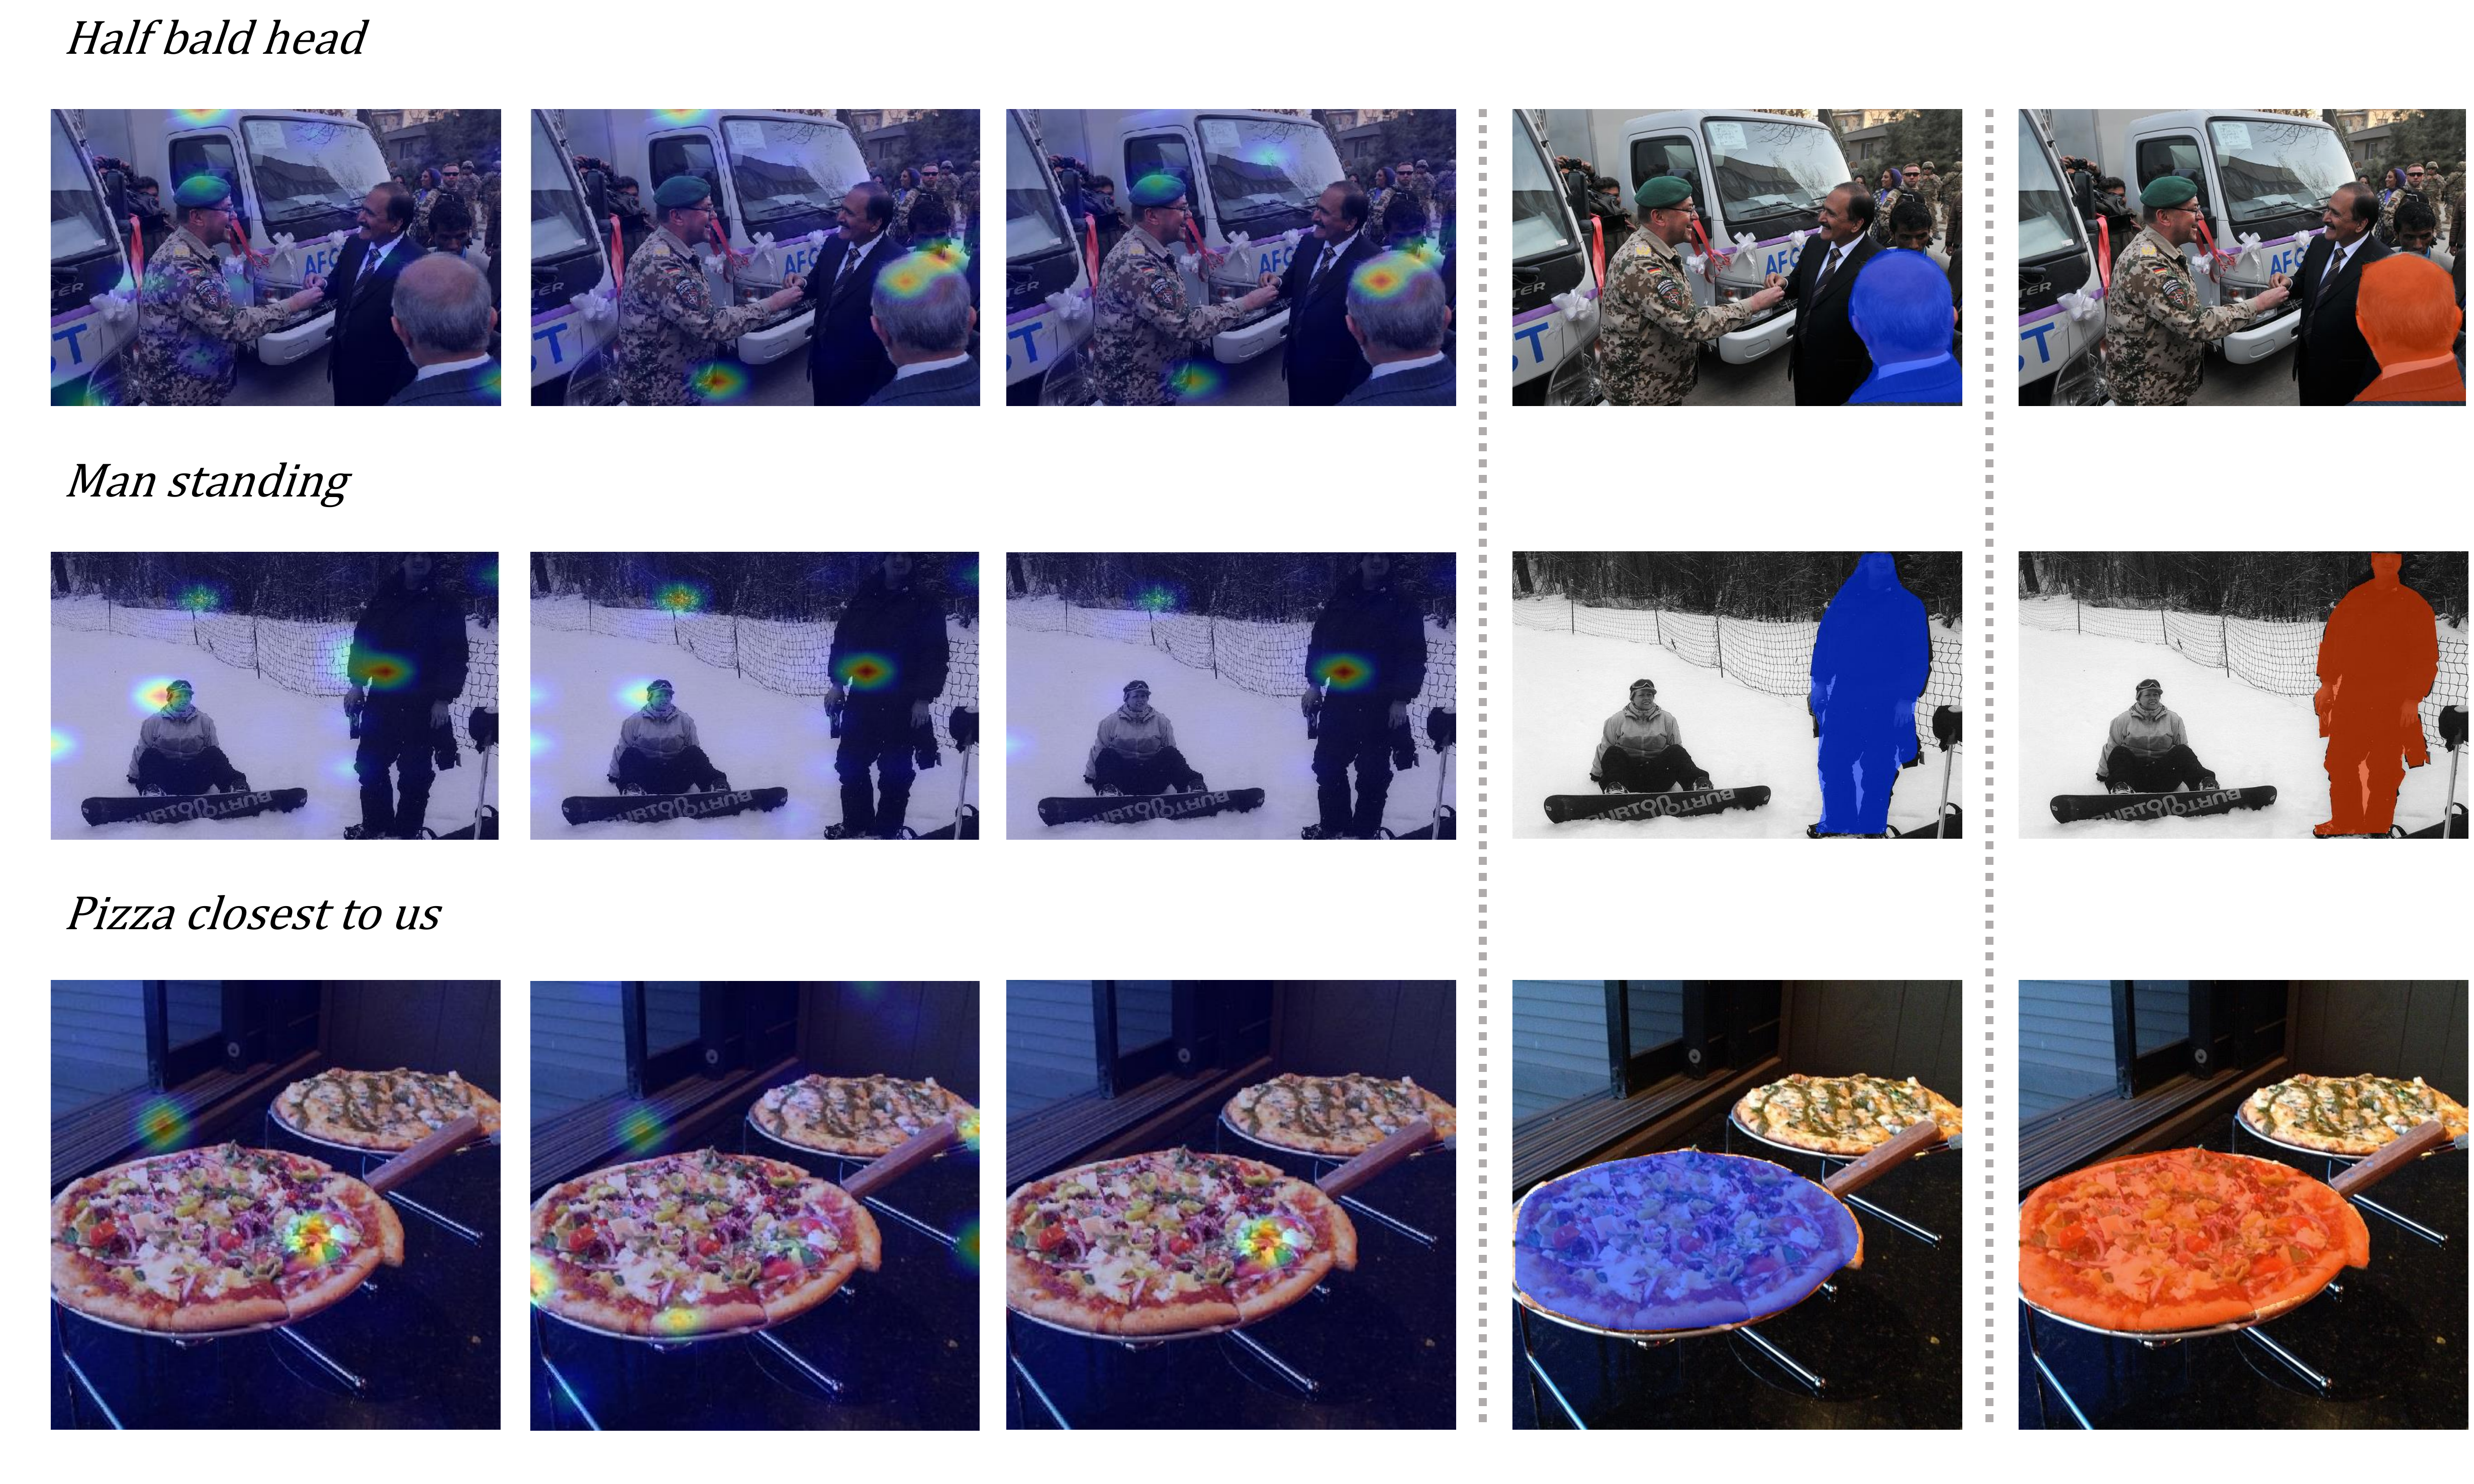}
  \vspace{0.1cm} \\
  \caption{Left three columns show the visualization of the attention maps as the depth of transformer encoder increasing. The fourth column is the final prediction and the column on the right indicates the ground truth. It can be seen that the network's attention gradually focuses on the proper referent instance.}
  \label{fig:vis_attn}
\end{figure*}

% in IOU/P5/P6/P7/P8/P9
% ----------fix aspect ratio--------
% refcoco val:    70.13/81.80/77.29/70.05/53.57/19.01
% refcoco testA:  71.71/84.76/81.08/72.72/55.86/16.69
% refcoco testB:  66.92/76.66/70.69/62.75/49.06/21.59
% refcoco+ val:   62.23/72.35/67.79/60.54/45.82/15.29
% refcoco+ testA: 65.92/77.81/73.17/65.22/48.89/13.75
% refcoco+ testB: 56.06/63.08/58.17/51.16/39.45/16.36
% refcocog val:   62.45/72.24/67.33/58.83/42.58/14.15
% refcocog test:  62.87/72.80/67.50/58.72/42.80/14.33
% refcocog-g val: 61.81/71.79/67.47/59.85/44.53/15.15

% ----------416 x 416--------
% refcoco val:    69.38/81.61/76.31/68.82/50.76/16.67
% refcoco testA:  71.31/84.35/79.81/71.86/54.22/14.92
% refcoco testB:  66.76/76.64/70.71/61.76/48.33/19.42
% refcoco+ val:   61.02/70.82/65.76/58.40/42.72/13.02
% refcoco+ testA: 64.68/75.92/71.00/63.15/47.22/12.86
% refcoco+ testB: 54.86/61.84/56.48/49.34/37.26/14.22
% refcocog val:   60.86/70.75/64.94/56.07/39.10/12.88
% refcocog test:  61.39/71.14/65.46/56.28/39.71/12.63
% refcocog-g val: 60.26/69.82/65.26/57.66/42.15/14.27
